# Supplementary material for: InteRACT: Transformer Models for Human Intent Prediction Conditioned on Robot Actions
Source: arXiv:2311.12943 source file (2024-06-02)
Supplement: Supplementary file 1 [file appendix.tex]

\appendix
% \section{Appendix}
\section{Appendix for ManiCast: Collaborative Manipulation with Cost-Aware Human Forecasting}
% \title{Appendix}

\textbf{Implementational Details} 
To test our framework, we provide 1 second of motion history as input to produce a 1 second forecast. We also follow \cite{Wang2021MultiPerson3M} and stack 3 layers of Transformer encoders (for both global and local-range) and the decoder. We use an Adam optimizer to train our models with weight decay of \SI{1e-5} and a multi-step learning rate scheduler with $\gamma = 0.1$ at milestones $[15, 25, 35, 40]$. Our starting learning rate is \SI{3e-4} for pre-training (batch size of 256) and \SI{1e-4} for fine-tuning (batch size of 64). We pre-train for 50 epochs and fine-tune for 30 epochs. We set $\lambda_{p} = 1$ and $\lambda_{h} = \lambda_{f} = 0.2$. We report metrics on human-human metrics on models where $J_H = 9$ upper body joints and human-robot metrics where $J_R = 2$ end effector positions. We also conduct experiments conditioning on 4 hand/wrist joints of the other human $C$ as opposed to all 9 joints, but find slightly better results and choose to focus our results on models conditioning on all of $J_H$. 

\begin{table*}[t!]
\centering
\resizebox{\textwidth}{!}
{
\begin{tabular}{ccccccccccc}
\toprule
% & Models $\xrightarrow{}$  & \multicolumn{2}{c}{\textsc{Baselines}} && \multicolumn{6}{c}{\textsc{Learning-Based}}\\  \cmidrule{3-4} \cmidrule{6-11}
& Metrics (mm) $\downarrow$  & {\textsc{Only PreTrain}} & {\textsc{Only FineTune}} & {\textsc{Marginal}} &{\textsc{Marginal-AllHist} \cite{Wang2021MultiPerson3M}} & {\textsc{InteRACT}}\\   
% & & ADE & FDE && ADE & FDE  && ADE & FDE && ADE & FDE && ADE & FDE && ADE & FDE && ADE & FDE && ADE & FDE\\
\midrule
\parbox[t]{2pt}{\multirow{4}{*}{\rotatebox[origin=c]{90}{\textsc{\scriptsize{ReactStir}}}}}
&All Joints FDE &97.7 (\pm 1.7) &68.5 (\pm 1.2) &59.5 (\pm 1.0) &61.0 (\pm 1.0) &\tbcolorg 53.7 (\pm 0.8) \\
&Hands/Wrists FDE &139.2 (\pm 2.4) &95.0 (\pm 1.6) &82.4 (\pm 1.3) &84.5 (\pm 1.3) &\tbcolorg 72.9 (\pm 1.1) \\
&T-All Joints FDE &95.9 (\pm 4.4) &66.5 (\pm 2.9) &60.4 (\pm 2.5) &61.5 (\pm 2.6) &\tbcolorg 54.4 (\pm 2.4) \\
&T-Hands/Wrists FDE &131.4 (\pm 6.1) &91.6 (\pm 4.0) &83.9 (\pm 3.5) &83.8 (\pm 3.6) &\tbcolorg 72.3 (\pm 3.3) \\
\midrule
\parbox[t]{2}{\multirow{4}{*}{\rotatebox[origin=c]{90}{\textsc{\scriptsize{Handover}}}}}
&All Joints FDE &89.4 (\pm 1.3) &68.3 (\pm 1.1) &62.0 (\pm 1.0) &62.0 (\pm 1.0) &\tbcolorg 57.5 (\pm 0.9) \\
&Hands/Wrists FDE &128.6 (\pm 2.0) &95.5 (\pm 1.5) &86.7 (\pm 1.4) &86.3 (\pm 1.4) &\tbcolorg 79.5 (\pm 1.3) \\
&T-All Joints FDE &124.7 (\pm 3.9) &92.4 (\pm 4.4) &86.3 (\pm 4.4) &86.0 (\pm 4.4) &\tbcolorg 79.7 (\pm 4.4) \\
&T-Hands/Wrists FDE &180.9 (\pm 6.8) &134.7 (\pm 6.8) &128.1 (\pm 6.9) &125.2 (\pm 6.7) &\tbcolorg 116.1 (\pm 6.6) \\
\midrule
\parbox[t]{2}{\multirow{2}{*}{\rotatebox[origin=c]{90}{\textsc{\scriptsize{Table}}}}}
&All Joints FDE &152.5 (\pm 1.1) &119.7 (\pm 0.9) &112.7 (\pm 0.8) &111.5 (\pm 0.8) &\tbcolorg 107.2 (\pm 0.8) \\
&Hands/Wrists FDE &195.4 (\pm 1.4) &153.8 (\pm 1.1) &146.0 (\pm 1.0) &144.3 (\pm 1.0) &\tbcolorg 138.9 (\pm 1.0) \\
\midrule
\parbox[t]{2}{\multirow{2}{*}{\rotatebox[origin=c]{90}{\textsc{\scriptsize{Avg.}}}}}
&All Joints FDE &124.2 (\pm 0.8) &94.9 (\pm 0.6) &87.6 (\pm 0.6) &87.3 (\pm 0.6) &\tbcolorg 82.2 (\pm 0.6) \\
&Hands/Wrists FDE &165.9 (\pm 1.1) &125.5 (\pm 0.8) &116.2 (\pm 0.8) &115.8 (\pm 0.7) &\tbcolorg 108.5 (\pm 0.7) \\
\bottomrule
\end{tabular}
}

\caption{Average forecast metrics (in mm) for all models across all CoMaD Human-Human datasets.}
\label{tab:forecasting_metrics}
\end{table*}

\begin{table*}[t!]
\centering
\resizebox{\textwidth}{!}
{
\begin{tabular}{ccccccccccc}
\toprule
% & Models $\xrightarrow{}$  & \multicolumn{2}{c}{\textsc{Baselines}} && \multicolumn{6}{c}{\textsc{Learning-Based}}\\  \cmidrule{3-4} \cmidrule{6-11}
& Metrics (mm) $\downarrow$  & {\textsc{Only PreTrain}} & {\textsc{Only FineTuned}} & {\textsc{Marginal}} & {\textsc{InteRACT}} & {\textsc{InteRACT + Align}}\\   
% & & ADE & FDE && ADE & FDE  && ADE & FDE && ADE & FDE && ADE & FDE && ADE & FDE && ADE & FDE && ADE & FDE\\
\midrule
\parbox[t]{2}{\multirow{2}{*}{\rotatebox[origin=c]{90}{\textsc{\scriptsize{Cab.}}}}}
&All Joints FDE &123.6 (\pm 2.4) &71.5 (\pm 1.7) &65.8 (\pm 1.6) &65.0 (\pm 1.6) &62.5 (\pm 1.5)\\
&Hands/Wrists FDE &155.3 (\pm 3.1) &87.4 (\pm 2.2) &79.4 (\pm 2.0) &77.8 (\pm 1.9) &75.2 (\pm 1.9)\\
\midrule
\parbox[t]{2}{\multirow{2}{*}{\rotatebox[origin=c]{90}
{\textsc{\scriptsize{Table}}}}}
&All Joints FDE &82.9 (\pm 1.9) &47.9 (\pm 1.2) &45.2 (\pm 1.4) &42.9 (\pm 1.3) &42.5 (\pm 1.3)\\
&Hands/Wrists FDE &97.1 (\pm 2.1) &54.4 (\pm 1.4) &51.1 (\pm 1.6) &47.5 (\pm 1.4) &46.8 (\pm 1.4)\\
\midrule
\parbox[t]{2}{\multirow{2}{*}{\rotatebox[origin=c]{90}
{\textsc{\scriptsize{Cart}}}}}
&All Joints FDE &97.1 (\pm 2.1) &58.3 (\pm 1.4) &50.2 (\pm 1.2) &49.8 (\pm 1.3) &49.3 (\pm 1.2)\\
&Hands/Wrists FDE &109.1 (\pm 2.2) &64.4 (\pm 1.6) &56.1 (\pm 1.4) &55.1 (\pm 1.4) &54.6 (\pm 1.4)\\
\midrule
\parbox[t]{2}{\multirow{2}{*}{\rotatebox[origin=c]{90}
{\textsc{\scriptsize{Avg.}}}}}
&All Joints FDE &102.8 (\pm 1.3) &60.3 (\pm 0.9) &54.4 (\pm 0.8) &53.4 (\pm 0.8) &52.2 (\pm 0.8)\\
&Hands/Wrists FDE &122.3 (\pm 1.6) &69.9 (\pm 1.1) &63.0 (\pm 1.0) &61.1 (\pm 1.0) &59.9 (\pm 1.0)\\
\bottomrule
\end{tabular}
}

\caption{Average forecast metrics (in mm) for all models across all CoMaD Human-Robot datasets.}
\label{tab:forecasting_metrics_hr}
\end{table*}

\begin{table}[t!]
\centering

\begin{tabular}{ccc}
\toprule
FDE (in mm) $\rightarrow$ & All Joints & Wrist and Hand \\
\midrule
% {\textsc{Marginal} - Only AMASS} & $417.2 (\pm 22.6)$ & $461.2 (\pm 22.3)$\\
{\textsc{Only FineTuned} & $424.9 (\pm 25.8)$& $446.3 (\pm 24.1)$\\
{\textsc{Marginal}} & $416.4 (\pm 24.1)$& $442.7 (\pm 23.0)$\\
\textsc{Marginal} (+ Hist) \cite{Wang2021MultiPerson3M} & $414.0 (\pm 23.9)$ & $444.7 (\pm 23.0)$\\
{\textsc{InteRACT} (ours)} & $\mathbf{412.6 (\pm 21.2)}$& $\mathbf{437.5 (\pm 20.0)}$\\
\bottomrule
\end{tabular}

\caption{Average prediction metrics (in mm) for all models on the CMU-MoCap dataset.}
\label{table:forecasting_metrics_cmu}
\end{table}

% \begin{table*}[t!]
% \centering
% \resizebox{\textwidth}{!}
% {
% \begin{tabular}{ccccccccccc}
% \toprule
% % & Models $\xrightarrow{}$  & \multicolumn{2}{c}{\textsc{Baselines}} && \multicolumn{6}{c}{\textsc{Learning-Based}}\\  \cmidrule{3-4} \cmidrule{6-11}
% & Metrics (mm) $\downarrow$  & {\textsc{Only PreTrain}} & {\textsc{Only FineTune}} & {\textsc{Marginal}} &{\textsc{Marginal-AllHist} \cite{Wang2021MultiPerson3M}} & {\textsc{InteRACT}}\\   
% % & & ADE & FDE && ADE & FDE  && ADE & FDE && ADE & FDE && ADE & FDE && ADE & FDE && ADE & FDE && ADE & FDE\\
% \midrule
% \parbox[t]{2}{\multirow{2}{*}{\rotatebox[origin=c]{90}{\textsc{\scriptsize{CMU}}}}}
% &All Joints FDE &417.2 (\pm 22.6) &424.9 (\pm 25.8) &416.4 (\pm 24.1) &445.9 (\pm 25.3) &\tbcolorg 412.6 (\pm 21.2) \\
% &Hands/Wrists FDE &461.2 (\pm 22.3) &446.3 (\pm 24.1) &442.7 (\pm 23.0) &472.8 (\pm 23.8) &\tbcolorg 437.5 (\pm 20.0) \\
% \bottomrule
% \end{tabular}
% }

% \caption{Average forecast metrics (in mm) for all models on the CMU-MoCap dataset.}
% \label{tab:forecasting_metrics_cmu}
% \end{table*}

% \input{tables/table3}
